# Supplementary material for: Strain-tunable orbital, spin-orbit, and optical properties of monolayer transition-metal dichalcogenides
Source: arXiv:1909.10763 source file (2019-11-19)
Supplement: Supplementary file 1 [file supplement.pdf]

# Supplemental Material:
# Strain-tunable orbital, spin-orbit, and optical properties of monolayer transition-metal dichalcogenides

Klaus Zollner,[1,*] Paulo E. Faria Junior,[1] and Jaroslav Fabian[1]

[1] *Institute for Theoretical Physics, University of Regensburg, 93040 Regensburg, Germany*

In the Supplemental Material we show fit parameters for $WS_2$, $MoSe_2$, and $WSe_2$ as function of biaxial strain. Furthermore, we compare the results for $MoS_2$, $WS_2$, $MoSe_2$, and $WSe_2$ when using a different functional in the first-principles calculations.

## S1. FITTING PARAMETERS FOR OTHER TMDCS

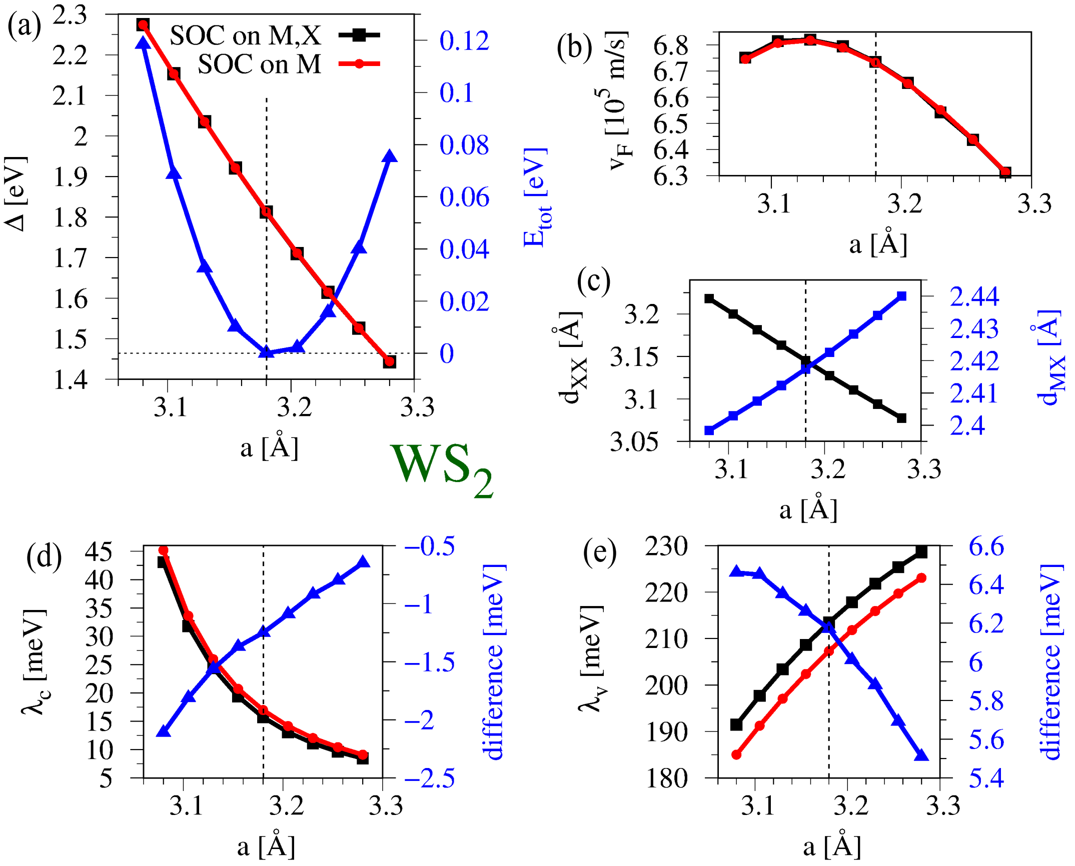


FIG. S1. (Color online) Summary of the fit parameters for $WS_2$ as a function of the lattice constant. (a) The gap parameter $\Delta$ and the total energy $E_{tot}$. The black data (SOC on M,X) correspond to calculations where SOC is included for both atoms M and X, while for the red data (SOC on M), we turned off SOC on the X atoms, respectively. Dashed vertical lines indicate the equilibrium lattice constant. (b) The Fermi velocity $v_F$. (c) The distances $d_{XX}$ and $d_{MX}$. (d,e) The SOC parameters $\lambda_c$ and $\lambda_v$. The difference (blue curve) is between the black and the red cure.

Similar to Fig. 4 of the main manuscript, we show the fit parameters for $WS_2$, $MoSe_2$, and $WSe_2$ in Figs. S1, S2, and S3. The observed dependence of the fit parameters, total energies, and distances on the lattice constant are similar to the case of $MoS_2$, shown in the main manuscript.

* klaus.zollner@physik.uni-regensburg.de

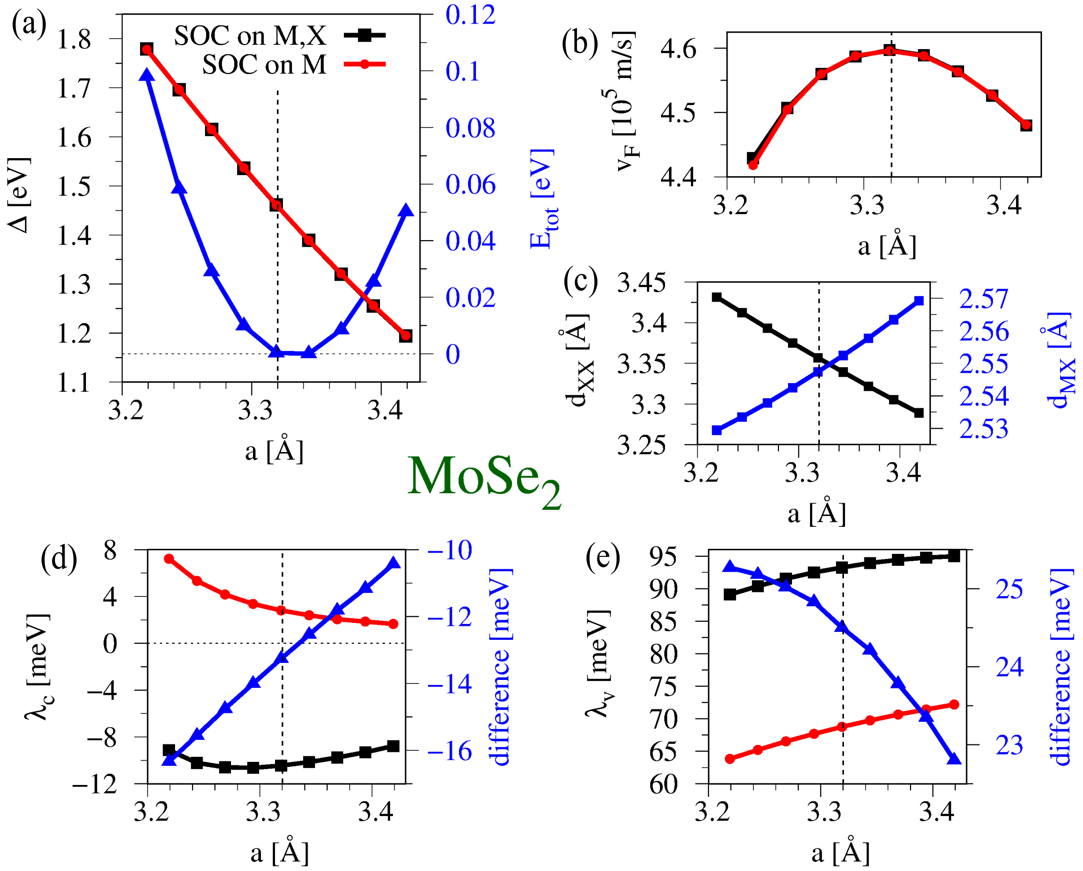


FIG. S2. (Color online) Same as Fig. S1, but for $MoSe_2$.

Comparing all four TMDC cases, we note that heavier elements (W, Se) give a larger contribution to spin-orbit band splittings than the lighter elements (Mo, S). For example, comparing Figs. S1(e) and S3(e), we find that the contribution from the Se atom to the VB SOC parameter is about 20 meV, while the one of the S atom is only about 6 meV.

## S2. COMPARISON OF PBE AND PBESOL FUNCTIONAL

In Fig. S4, we compare the results from PBE [1] to the ones from PBEsol [2] exchange correlation functional, for the case of $MoS_2$. We find that the equilibrium lattice constant from PBEsol is $a = 3.15$ Å, in very good agreement with experiment, while PBE, giving $a = 3.185$ Å, overestimates the experimental lattice constant by about 1%. However, the trends that we observe for the fit parameters, as function of the lattice constant, are nearly the same for both functionals. Similarly, in Figs. S5, S6, and S7, we compare PBE and PBEsol functionals for $MoSe_2$, $WS_2$, and $WSe_2$. Again, the equilibrium lattice constant for PBEsol is in better agreement with the experimental value, but the general trends of all fit parameters are similar to the PBE functional.

We conclude that the PBEsol functional should hardly influence the results on exciton energy levels and gauge factors, and results can be compared to experiment, when regarding them relative to 0% strain (equilibrium lattice constant).


[1] J. P. Perdew, K. Burke, and M. Ernzerhof, Phys. Rev. Lett. **77**, 3865 (1996).

[2] J. P. Perdew, A. Ruzsinszky, G. I. Csonka, O. A. Vydrov, G. E. Scuseria, L. A. Constantin, X. Zhou, and K. Burke, Phys. Rev. Lett. **100**, 136406 (2008).

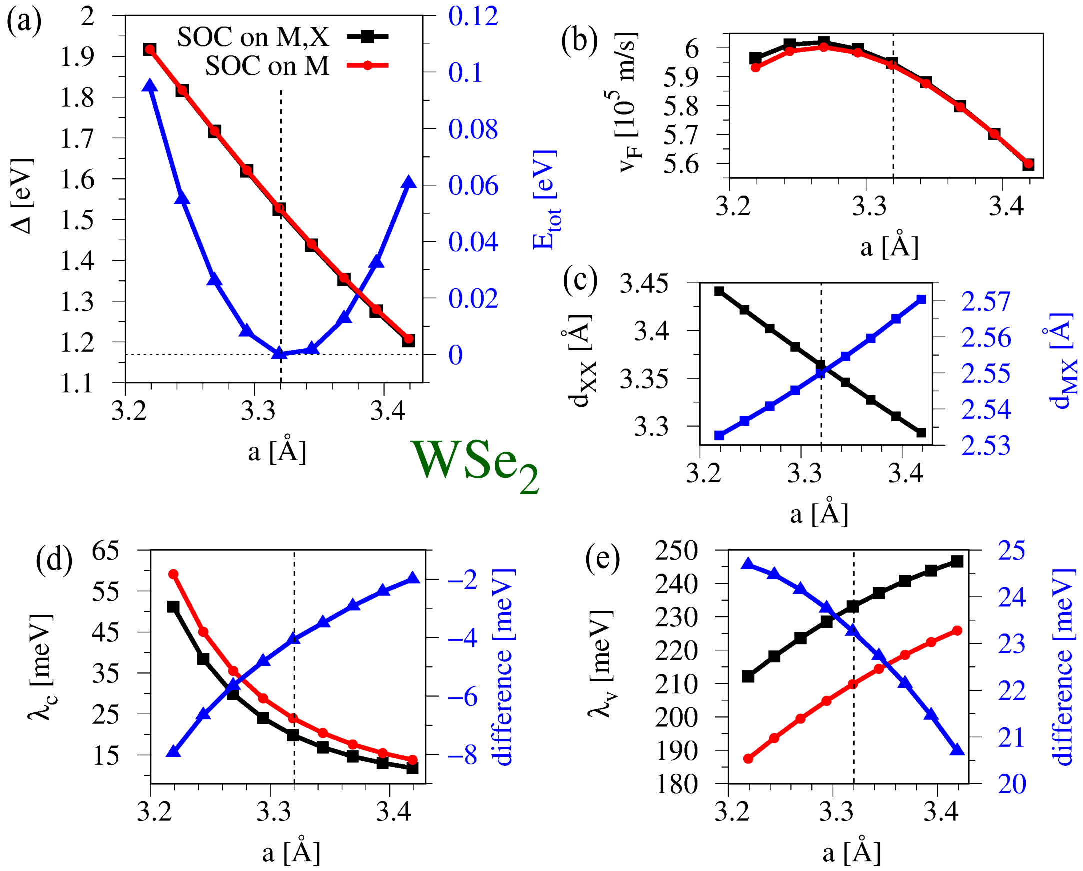


FIG. S3. (Color online) Same as Fig. S1, but for $WSe_2$.

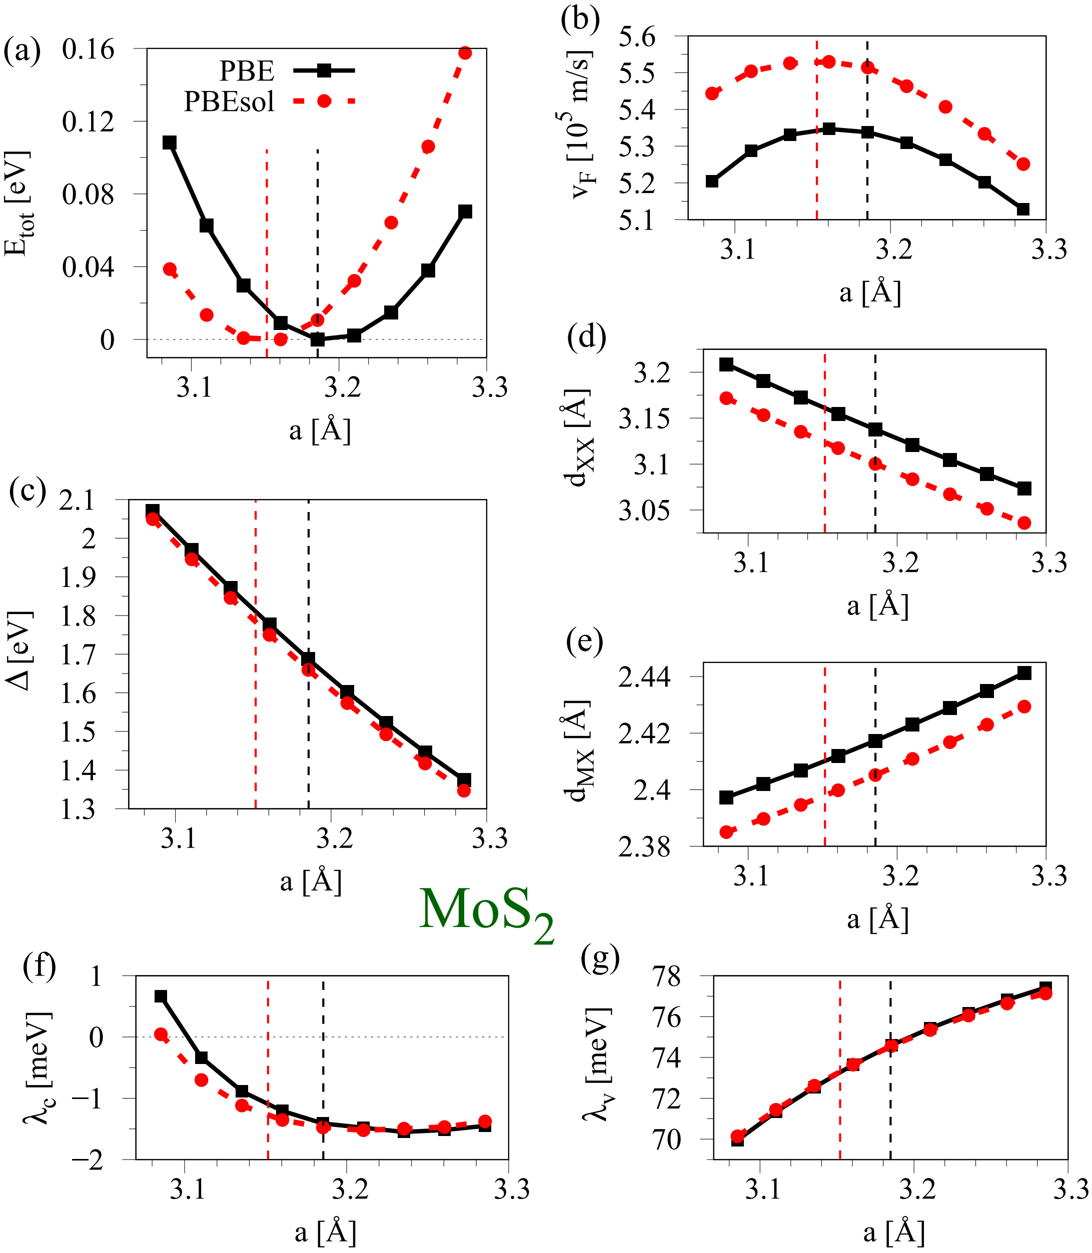


FIG. S4. (Color online) Comparison between the PBE (black squares) and PBEsol (red dots) functional for $MoS_2$ as function of the lattice constant. Dashed vertical lines indicate the equilibrium lattice constants. (a) Total energy $E_{tot}$, (b) the Fermi velocity $v_F$, (c) the gap parameter $\Delta$, (d,e) the distances $d_{XX}$ and $d_{MX}$, and (f,g) the SOC parameters $\lambda_c$ and $\lambda_v$.

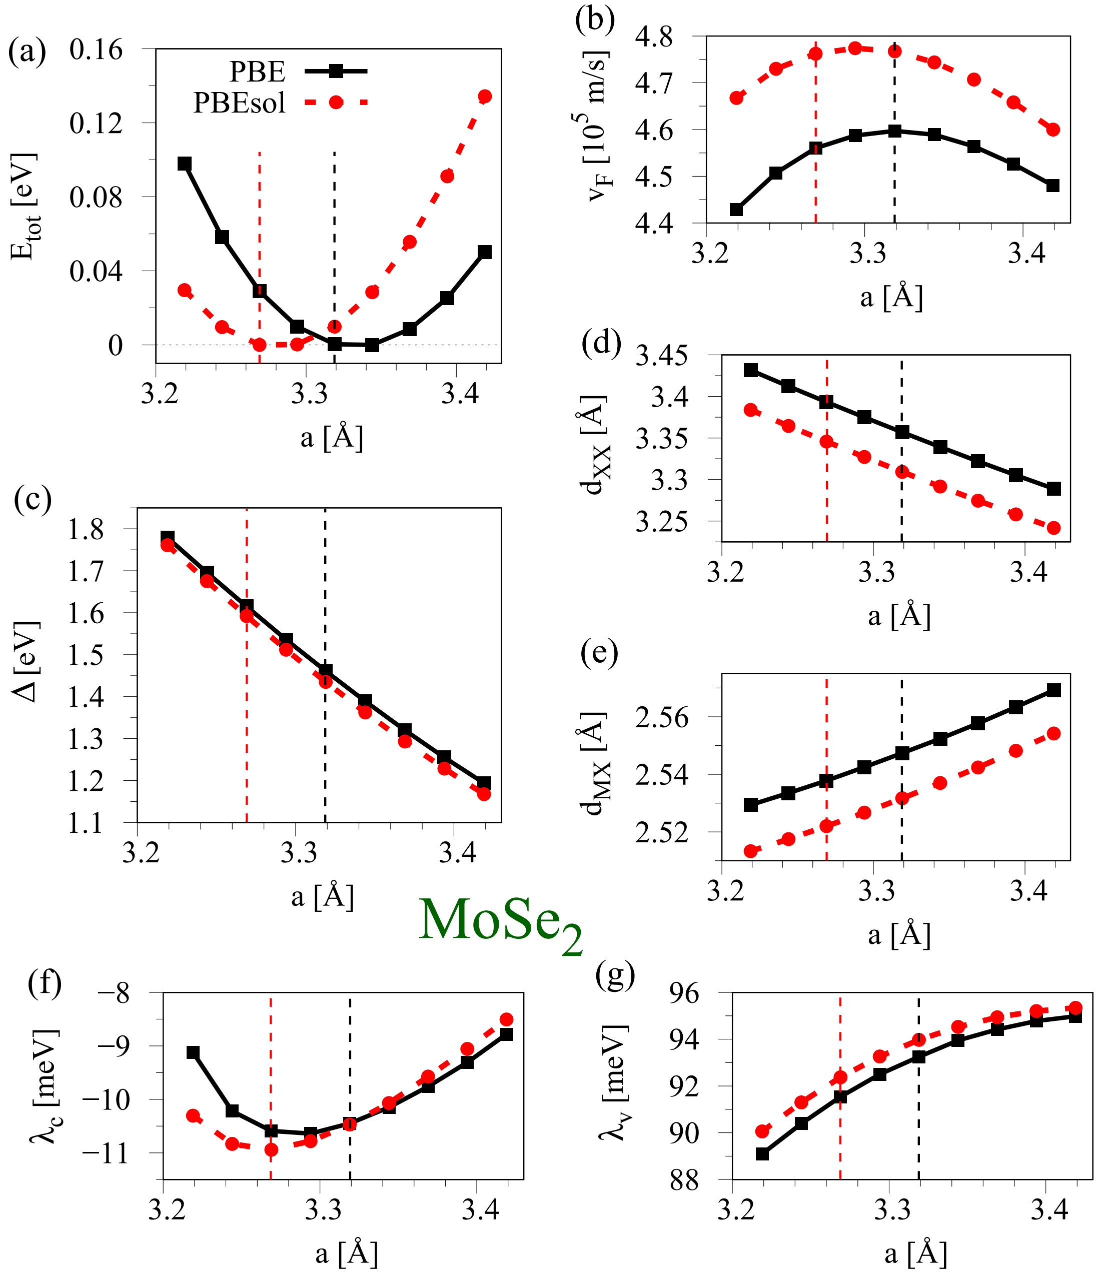


FIG. S5. (Color online) Same as Fig. S4, but for $MoSe_2$.

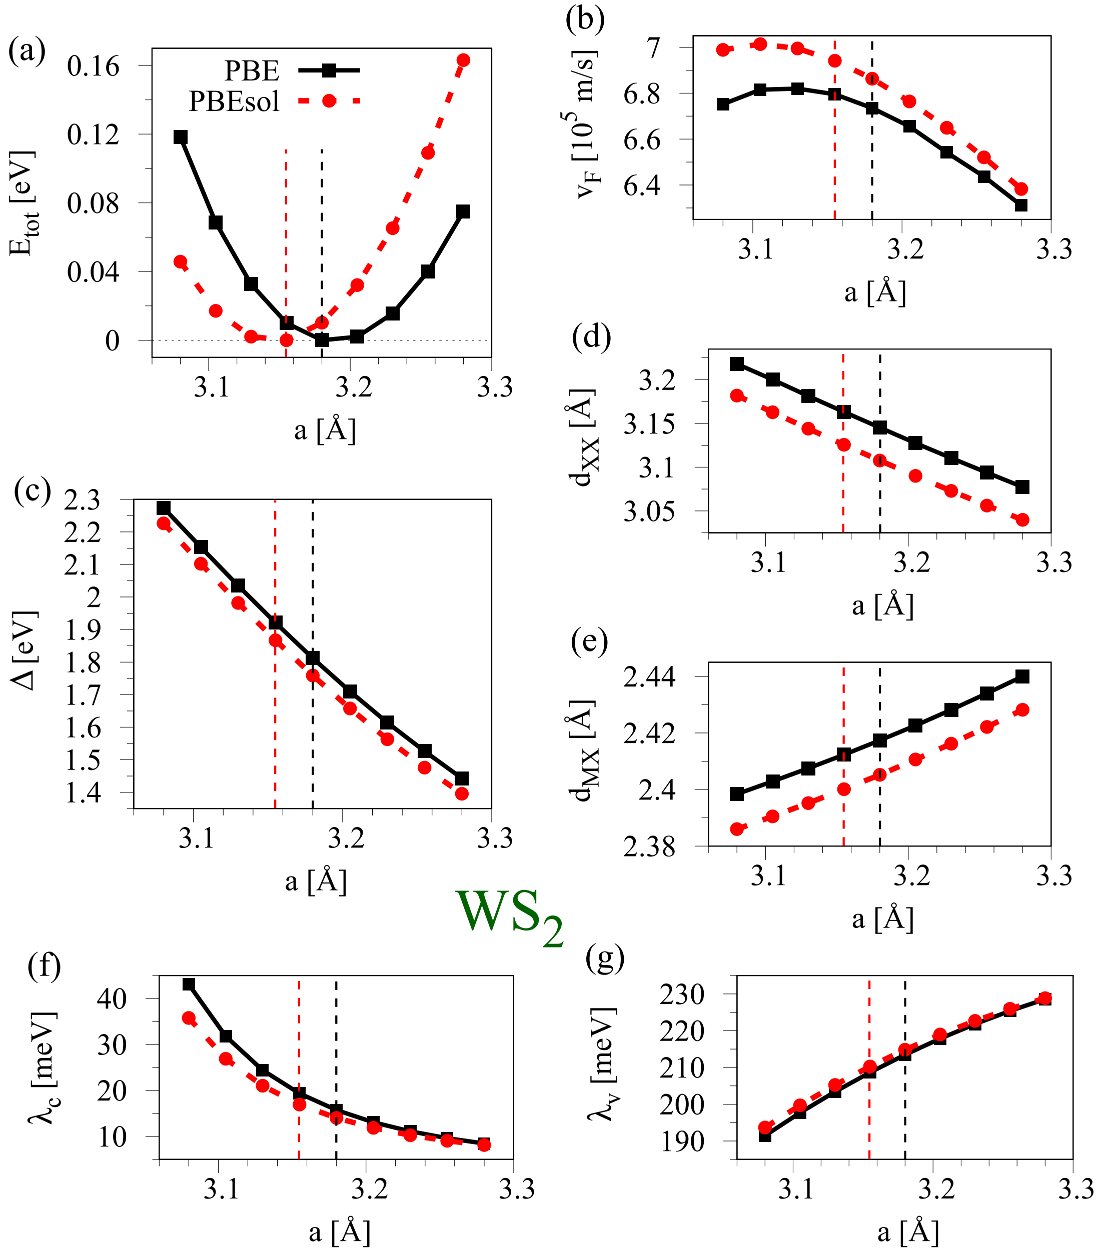


FIG. S6. (Color online) Same as Fig. S4, but for $WS_2$.

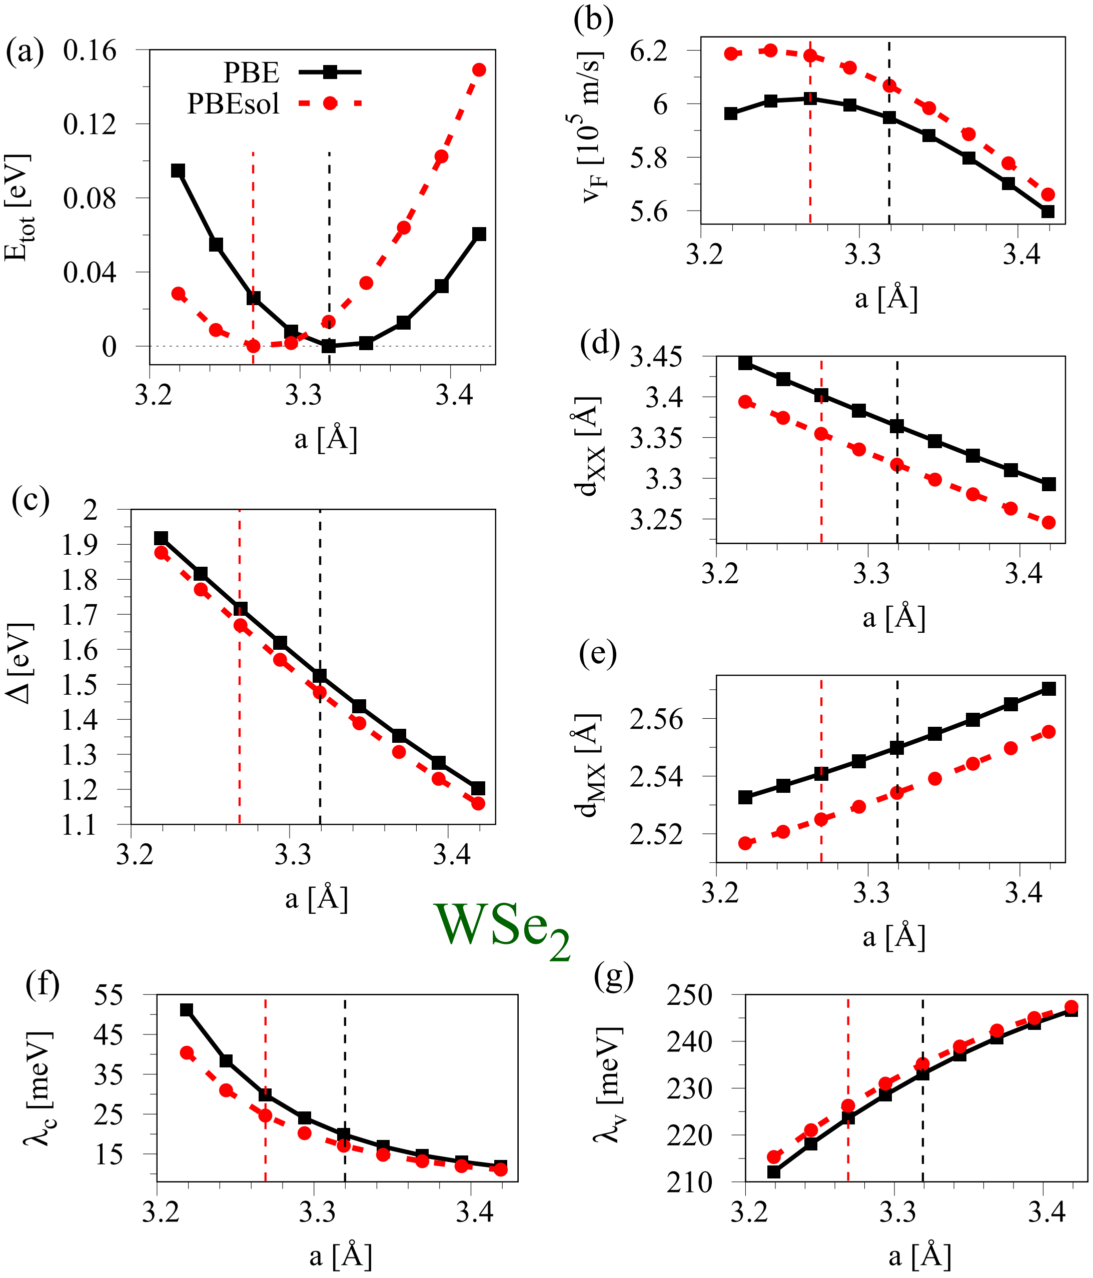


FIG. S7. (Color online) Same as Fig. S4, but for $WSe_2$.
